# Supplementary material for: Cross-correlation of DES Y3 lensing and ACT/${\it Planck}$ thermal Sunyaev Zel'dovich Effect I: Measurements, systematics tests, and feedback model constraints
Source: arXiv:2108.01600 source file (2021-08-03)
Supplement: Supplementary file 1 [file Appendix_IA.tex]

\section{Intrinsic alignments}\label{sect:IA}
\begin{figure*}
\includegraphics[width=1.\textwidth]{./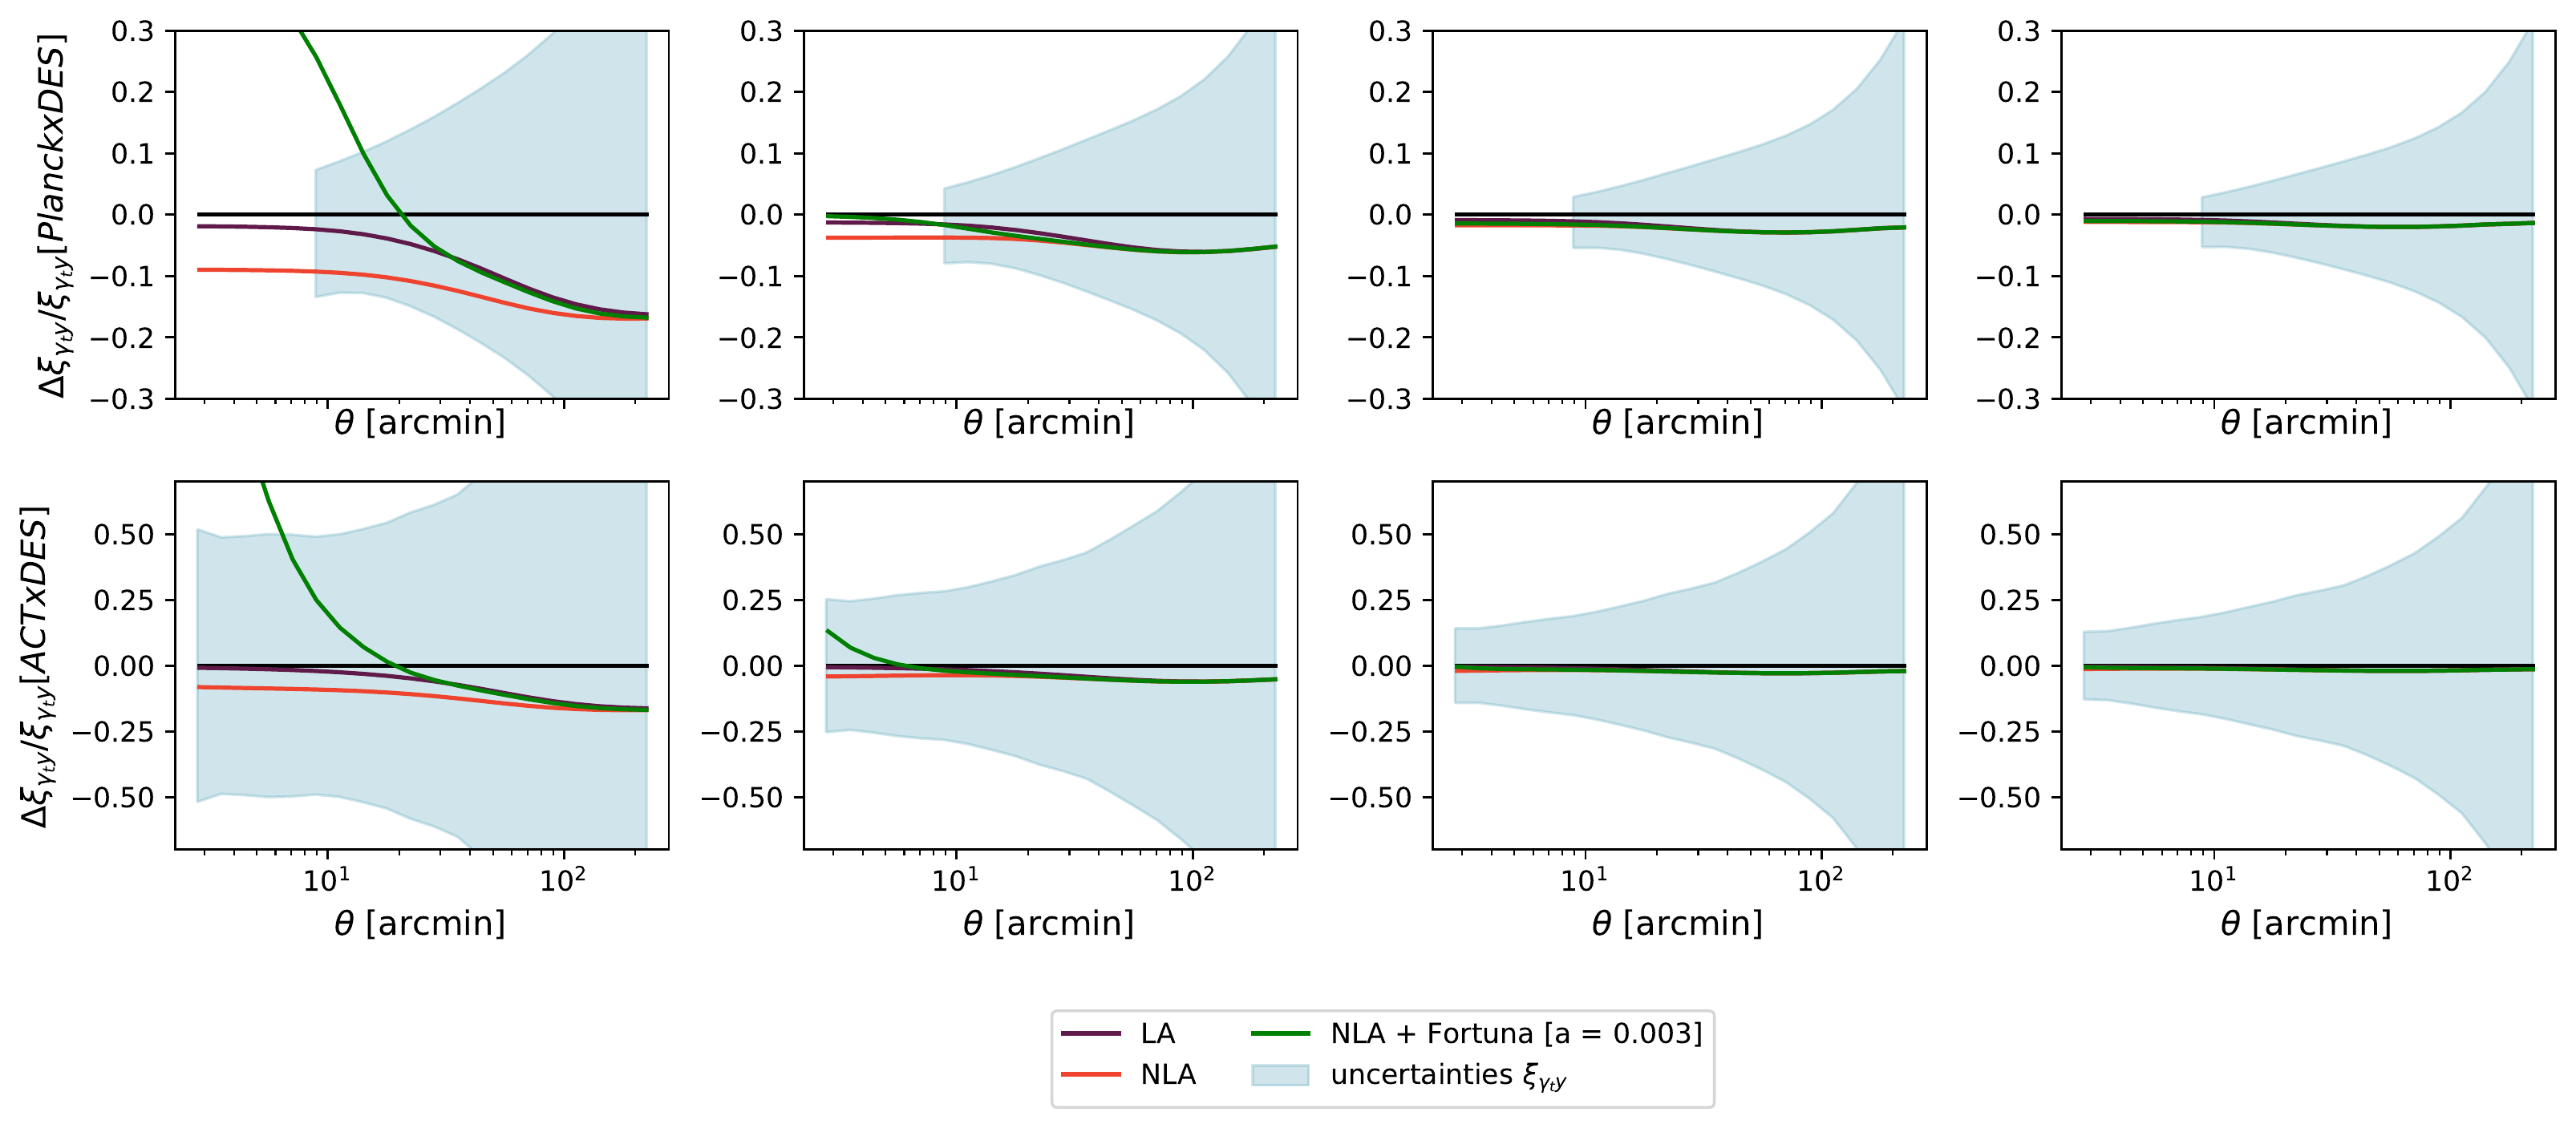}
\caption[]{Fractional difference in the data vector due to different IA models. In particular, we compare the linear alignment model (LA), the non linear alignment model (NLA) and the NLA model with the addition of the 1-halo IA contribution due to satellite galaxies alignment \citep{Fortuna2020}.}
\label{ia_effect}
\end{figure*}
\SP{I think this is better suited in the scale cuts section of paper2}
In our analysis we included the non-linear alignment (NLA) model \citep{Hirata2004,Bridle2007} for intrinsic galaxy alignments. The contribution to the shear-Compton-$y$ signal due to IA has been ignored so far, but as we discuss here, it can have a non negligible impact, especially at low redshift.

In Fig. \ref{ia_effect} we show the fraction difference with respect to a theory data vector due to different IA models. We considered three different IA models. The first one is the linear alignment model (LA); it is obtained by following eq. \ref{eq:ia_nla}, but only including the 2-halo contribution, i.e. the part proportional to the matter linear power spectrum. For the predictions shown in the Figure, we adopted best fit values from \cite{Samuroff2019} for the amplitude $A_{\rm IA,0}$, and fixed the redshift evolution parameter $\eta_{\rm IA}$ to 0. The non-linear alignment extension is usually obtained starting from LA by substituting the linear power spectrum with the non linear power spectrum. In our case, as we are modelling the correlation using the halo model formalism, the NLA part is modelled by including the 1-halo contribution to the shear-Compton-$y$ signal. For the predictions shown in the Figure, we also adopted best fit values from \cite{Samuroff2019} for the amplitude $A_{\rm IA,0}$, and fixed the redshift evolution parameter $\eta_{\rm IA}$ to 0. Last, we also show a more complex model that includes an additional 1-halo IA contribution due to satellite galaxies alignment, following \cite{Fortuna2020}.  This extra contribution requires modelling of the Halo Occupation Distribution (HOD) of satellite galaxies and the fraction of satellites as a function of redshift, which are somewhat uncertain for the DES Y3 weak lensing sample. For this reason, we decided to provide an order-of-magnitude estimate for this contribution, and remove scales where this extra 1-halo model could provide a significant contribution to our data vector. For the predictions shown in the Figure, we therefore adopted XXX \textbf{shivam needed}. The overall amplitude of the model is controlled by a parameter $a_{\rm 1h}$, which \cite{Fortuna2020} fix to $a_{\rm 1h} =0.001$. For our predictions, to be conservative, we adopted $a_{\rm 1h} =0.003$.

The main message that Fig. \ref{ia_effect} conveys is that IA can have a non negligible impact on our data vector at low redshift, for the first tomographic bin.  At large scales, given our measurement sensitivity, IA is probably relevant only for the first tomographic bin of the DES x \textit{Planck} measurement. At small scales, the 1-halo contribution from the \cite{Fortuna2020} model can have a drastic impact. Our estimates for that model are not driven by our data set, but they should be robust enough as upper limit. Based on this comparison we decided to exclude from our analysis scales smaller than 20 arcminutes for the first tomographic bin, and smaller than 5 arcminutes for the second tomographic bin. In such a way, we exclude the scales where the \cite{Fortuna2020} model might assume a relevant contribution.

We note that other IA models exist in literature. One major example is the tidal alignment and tidal torquing model (TATT, \citet{Blazek2019}), implemented in the main DES Y3 cosmological analysis \citep{DES2020}, which generalises over the NLA model. We did not implement the TATT model here, as a formulation compatible with the halo model framework does not exist. We note, however, that the main DES Y3 cosmological results obtained assuming either the TATT or NLA models were compatible with each other. For this reason, we consider the NLA model sufficiently adequate for this work.
