# Supplementary material for: Cross-correlation of DES Y3 lensing and ACT/${\it Planck}$ thermal Sunyaev Zel'dovich Effect I: Measurements, systematics tests, and feedback model constraints
Source: arXiv:2108.01600 source file (2021-08-03)
Supplement: Supplementary file 2 [file Appendix_radio_tests.tex]

\section{Systematic tests}\label{sect:map_tests}
\begin{figure*}
\includegraphics[width=1.\textwidth]{./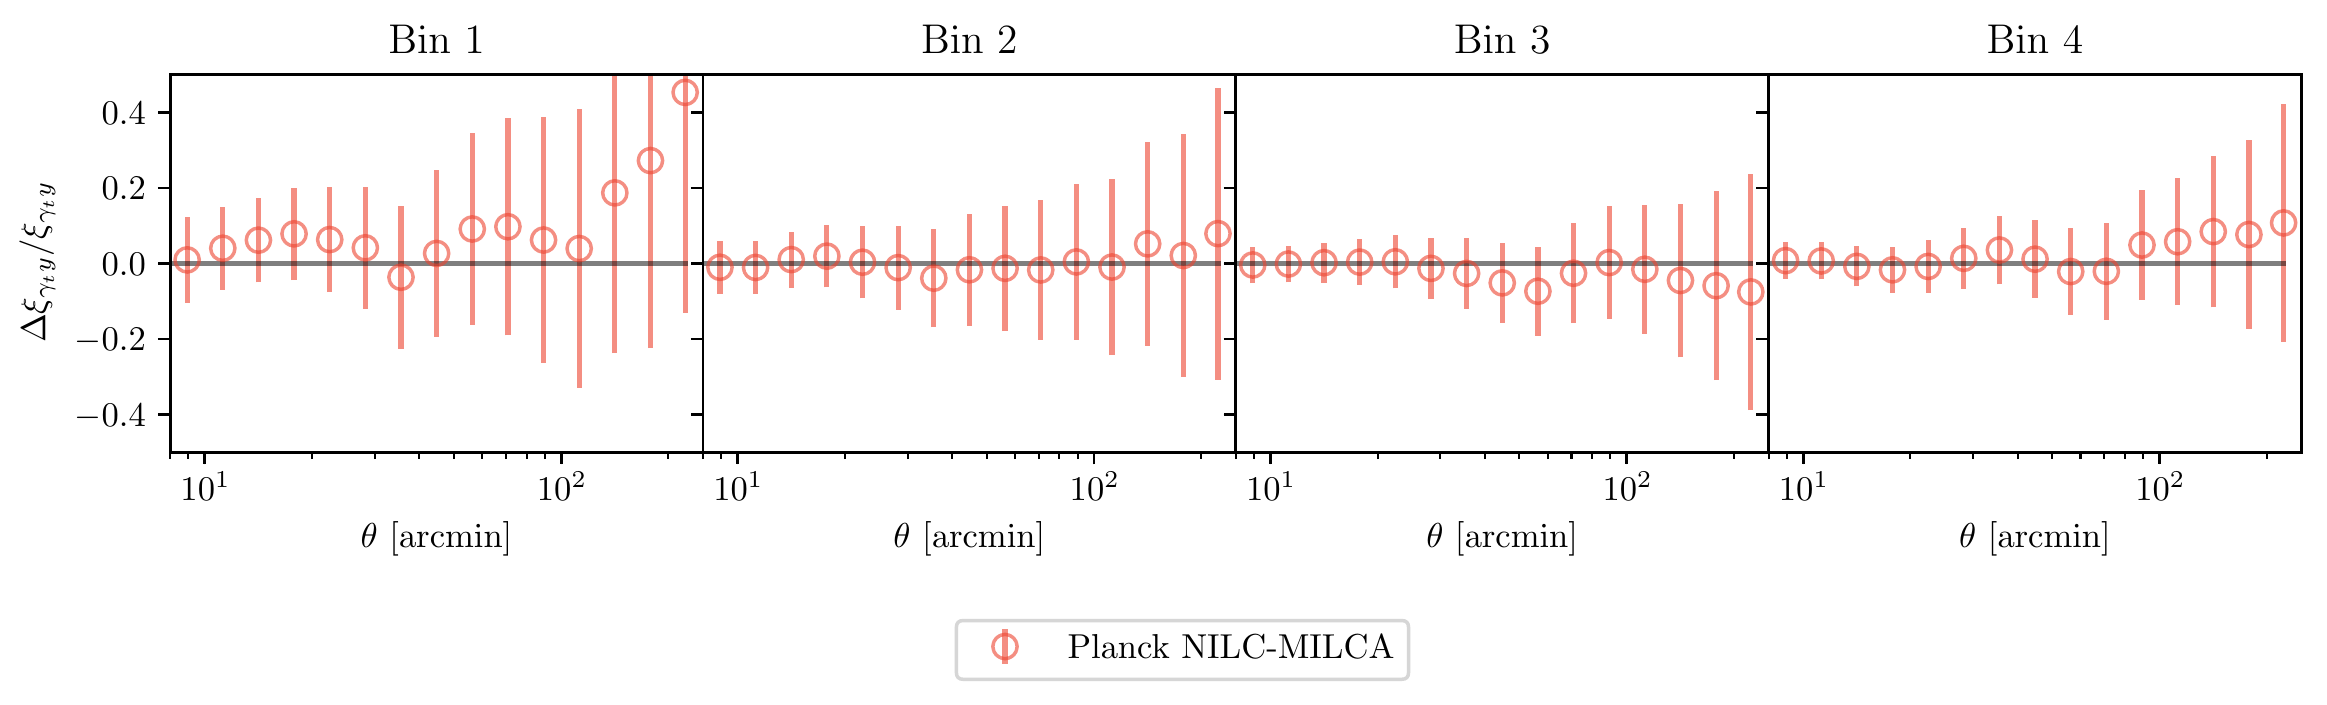}
\caption[]{Fractional difference in the measured shear-Compton-$y$ cross-correlation $\xi^{\gamma_t y}$ when computed using the \texttt{MILCA} and \texttt{NILC} \textit{Planck} Compton-$y$ maps.}
\label{measurement_planck_MILCA_NILCA}
\end{figure*}
\begin{figure*}
\includegraphics[width=1.\textwidth]{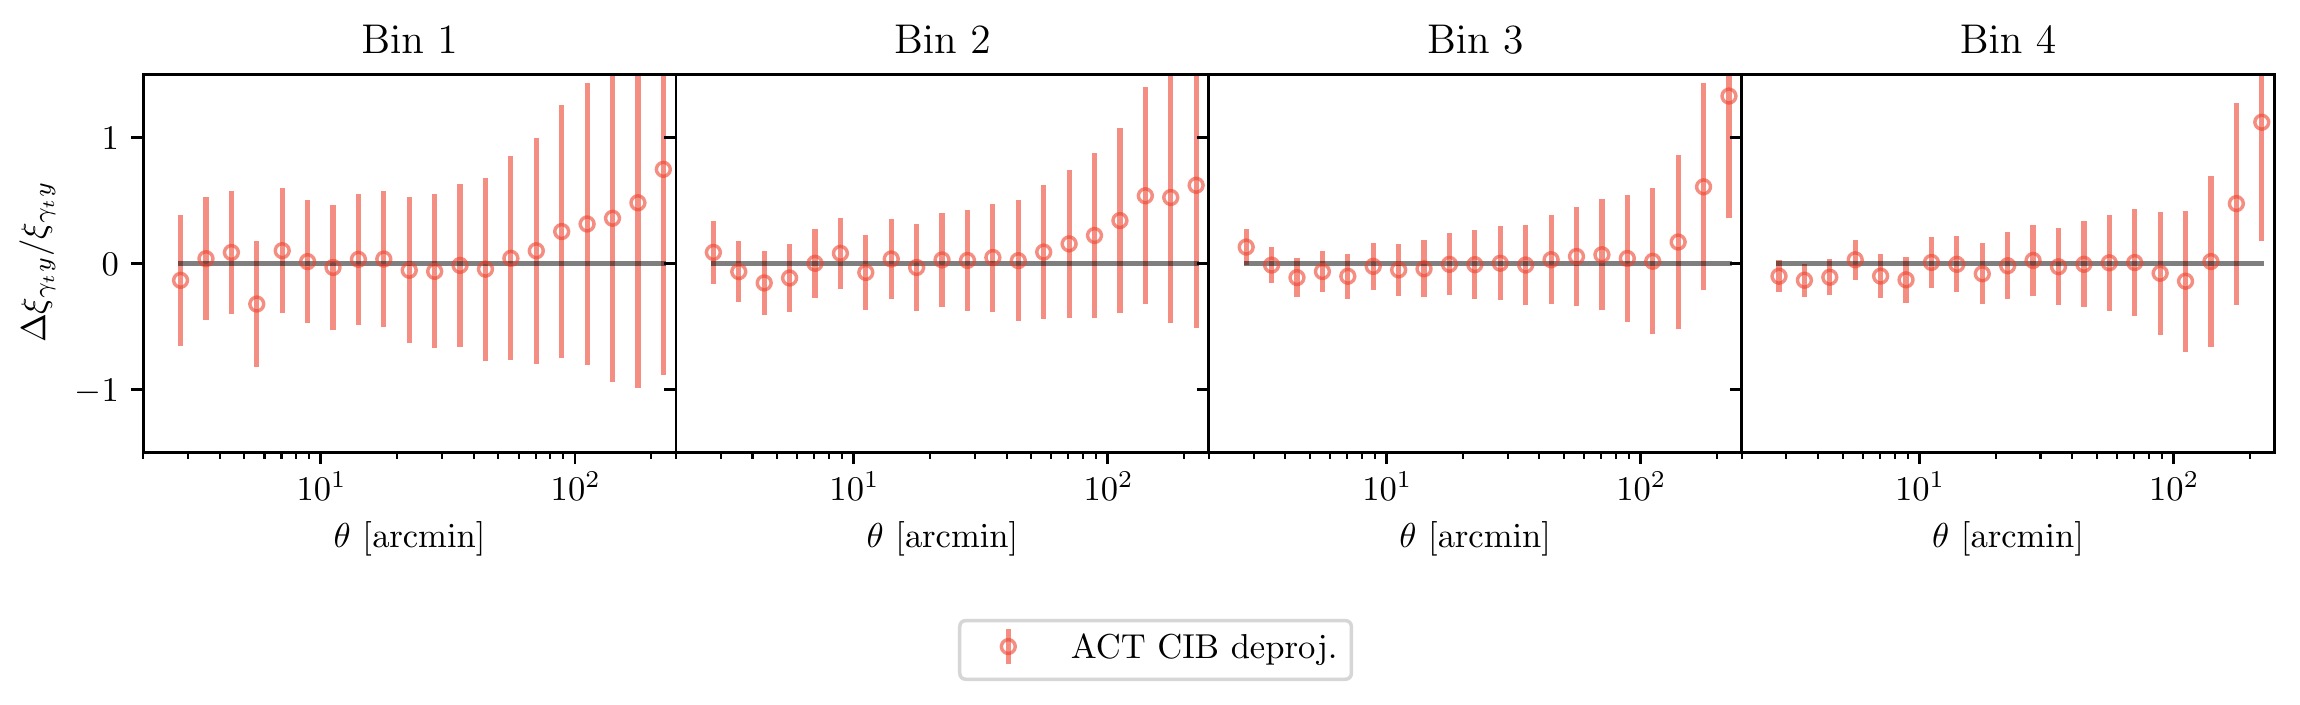}
\caption[]{Fractional difference in the measured shear-Compton-$y$ cross-correlation $\xi^{\gamma_t y}$ when computed using the ACT map after explicitly de-projecting CIB components.}
\label{measurement_act_cib_cmb}
\end{figure*}
\begin{figure*}
\includegraphics[width=1.\textwidth]{./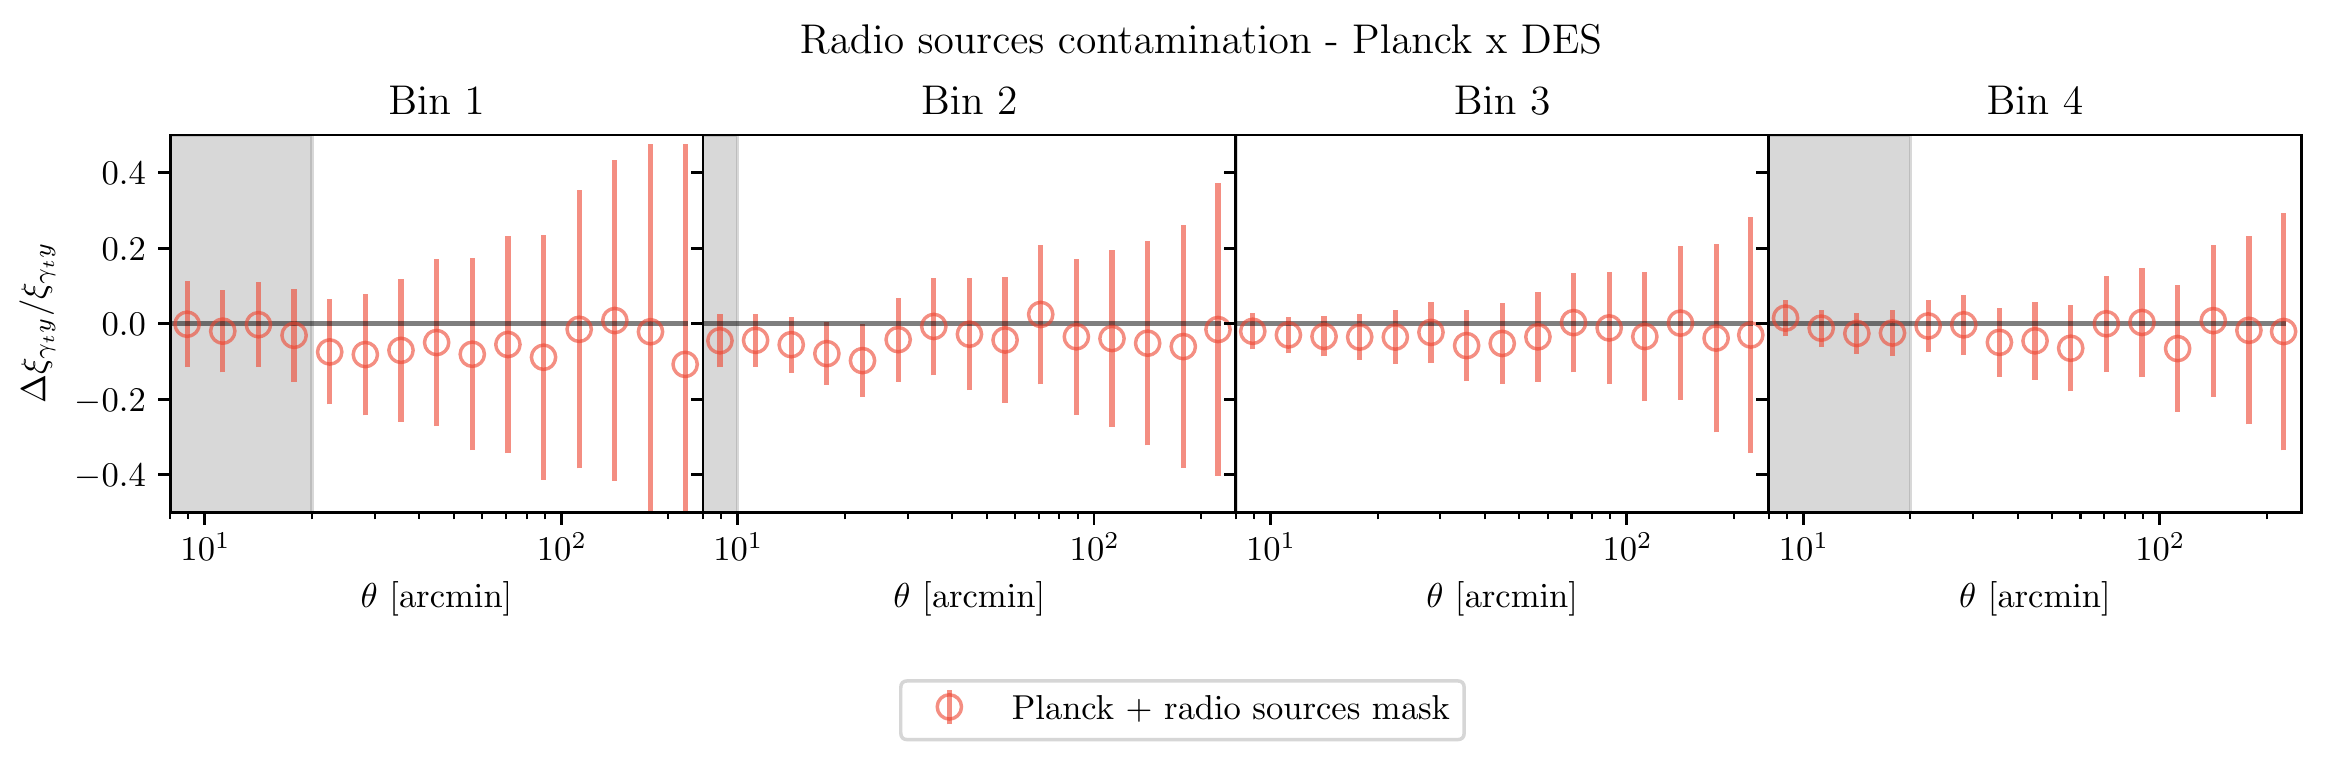}
\caption[]{Fractional difference in the measured shear-Compton-$y$ cross-correlation $\xi^{\gamma_t y}$ when computed using the \textit{Planck} Compton-$y$ map with and without masking radio sources.}
\label{measurement_planck_radio}
\end{figure*}
\begin{figure*}
\includegraphics[width=1.\textwidth]{./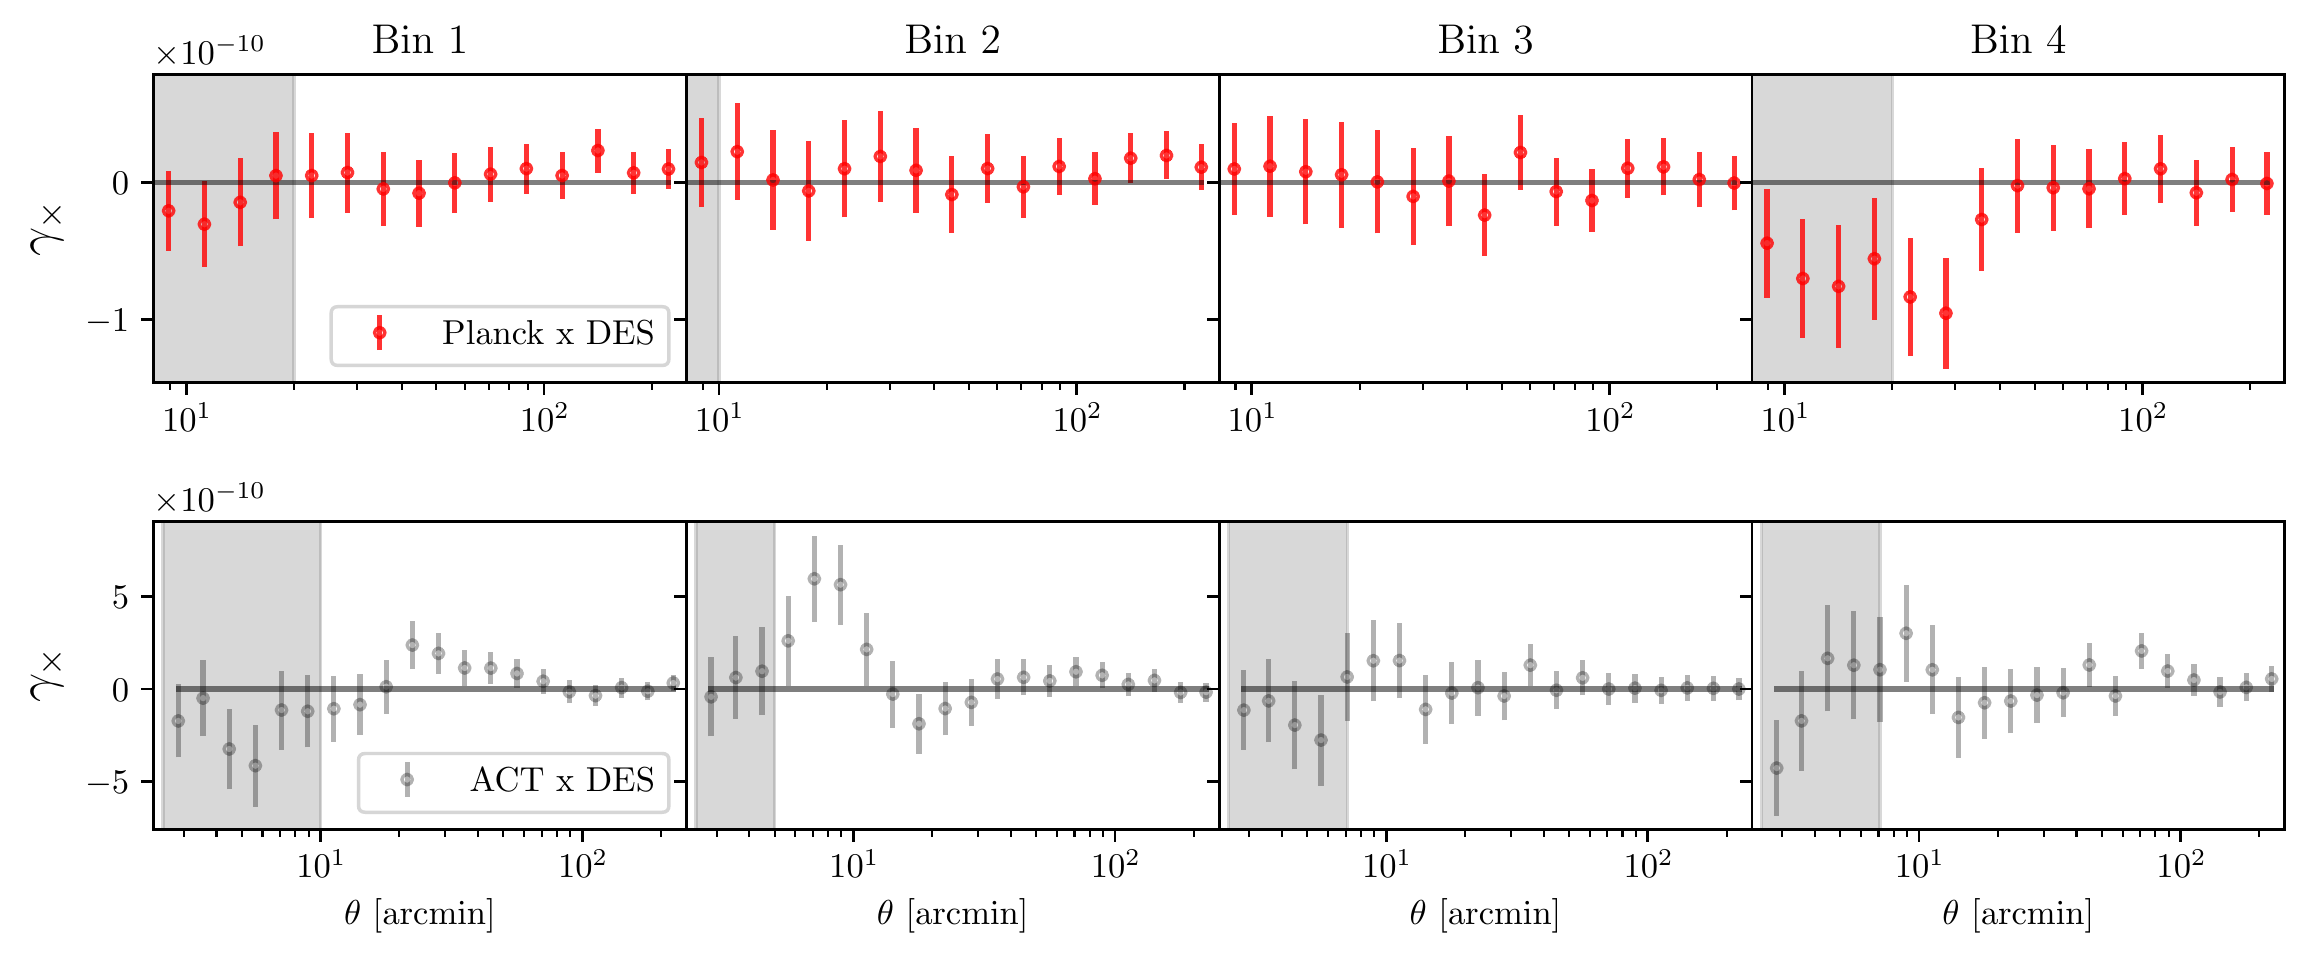}
\caption[]{Cross-component of the lensing signal around points of the Compton-$y$ maps.}
\label{cross_component}
\end{figure*}
Before analysing our measurements, we perform in this section a number of systematic tests. 

As a first test, we compare the $\xi^{\gamma_t y}(\theta)$ signal measured using two different versions of the \textit{Planck} Compton-$y$ maps, obtained with two slightly different algorithms, \texttt{MILCA} and \texttt{NILC} \citep{Planck_2016_tsz}. Both algorithms are based on the ILC method, which aims at finding the most optimal linear combination of maps from different frequency channels that minimises the variance of the final map, under the
constraint of offering unit gain to the frequency dependence of the tSZ effect. The fractional difference of the  $\xi^{\gamma_t y}(\theta)$ signal between the \texttt{MILCA} and \texttt{NILC} maps is shown in Fig.~\ref{measurement_planck_MILCA_NILCA}. The measurements obtained with the maps little differ from each other, and the pull (defined as $\Delta\xi^{\gamma_t y}/\sigma_{\xi^{\gamma_t y}}$) of the individual data points is generally smaller than 0.5 (except for two points at large scales in the first tomographic bin, with pull $\sim 0.7-0.8$). This is somewhat expected, as the two measurements should be largely covariant. To further test consistency, we computed the $\chi^2$ of the difference of the two signals; we estimated the covariance using jackknife and considered only scales where the jackknife covariance is known to be reliable, i.e., $\theta<40$ arcmin (see Appendix \ref{sec:covariance}). We obtained a p-value = 0.05 ($\chi^2=41/28$ $d.o.f.$), suggesting consistency. We did not repeat this test for the ACT map, as only one type of map has been produced (using a slightly different ILC-based algorithm).

As a second test, we assess the potential effect of contaminants. The Compton-$y$ maps can contain contributions due to foregrounds, namely, the cosmic infrared background (CIB) and radio point sources. The maps can also be contaminated by a residual CMB signal, if it has not been properly removed by the components separation algorithm. The ILC map making method allows to explicitly de-project potential contaminants, as long as their SED is known. We start investigating this by looking at the $\xi^{\gamma_t y}(\theta)$ signal measured using two different versions of the Compton-$y$ maps, obtained by de-projecting the CIB or CMB components, respectively. %Note that the CIB is mostly sourced by thermal emission from galaxies throughout the Universe; although the main contribution comes from galaxies  at $z>2$, 
For this test we only focus on the ACT map, as the \textit{Planck} Compton-$y$ maps has already proven robust against CIB and CMB contamination \citep{Yan2019}. The de-projected ACT measurements, compared to the fiducial measurement used in this work (which does not include any explicit de-projection), are shown in Fig.~\ref{measurement_act_cib_cmb}. If we only consider the angular scales passing our scale cut (Table~\ref{table_scale_cuts}), the pull of the individual data points is generally smaller than 1, except for a couple of points at the smallest scales for the correlations involving the highest redshift bins (3 and 4) for the CMB de-projected map. Similar to the previous case, we checked if the measurements with the de-projected maps were compatible with the fiducial measurement by computing the $\chi^2$ of the difference between the signals, using a jackknife covariance and focusing on scales $\theta<15$ (i.e., the scales where the ACT jackknife covariance can be considered reliable). We obtained a p-value = 0.5 ($\chi^2=28/32$ $d.o.f.$) and p-value = 0.18 ($\chi^2=39/32$ $d.o.f.$) for the CMB and CIB de-projected measurements, respectively. This suggests there is no indication of CMB or CIB contamination in the ACT Compton-$y$ map. 

To test the potential contamination due to radio sources, we proceed differently. It has been claimed radio sources could potentially bias the signal at the 10-20 per cent level \citep{Shirasaki_2018}, although the exact number depends on the SED and HOD of the radio sources, which are uncertain, and on the map making algorithm. Due to the uncertainties in the SED and HOD, the radio sources contamination cannot be easily de-projected as in the case of the CMB and CIB. The ACT map is created masking detected radio sources in every channel  \citep{Madhavacheril2020}; radio sources are usually detected down to 5-10 mJy. The fiducial \textit{Planck} maps used in this work do not have any radio sources mask applied by default. We therefore apply a radio sources mask to the \textit{Planck} Compton-$y$ map, using a catalog of radio sources detected by ACT at 98 and 150 GHz. Note that ACT can detect point-like radio sources much fainter than \textit{Planck}. We masked an area of 10 arcmin around each source, and repeated the cross correlation measurement with the DES shape catalog. The masking reduced by 8 per cent the area available for the cross correlation. The difference in the measurements (with and without radio sources mask applied) is shown in Fig.~\ref{measurement_planck_radio}. The difference in amplitude is sufficiently small to consider any potential radio contamination negligible (using the angular scales where the jackknife covariance is reliable, we obtained for the difference between the two signals $\chi^2/d.o.f$ = 30/28). %30.217024901182207 28 %Note that the signal with the radio sources masked is has a preferentially lower amplitude compared 

%Note that using such an aggressive masking we are also preferentially removing regions of the map where a positive is signal is expected, rather than removing the true radio source contamination.

Last, we checked the cross-component of the mean shear around every point of the Compton-$y$ maps. The cross-component is a standard null test in galaxy-galaxy lensing studies, as it should be compatible with zero if the shear is produced by gravitational lensing alone. The cross-component should also vanish in presence of systematic effects that are invariant under parity. We test this in Fig.~\ref{cross_component}. We obtain $\chi^2/d.o.f$ = 84/68 and $\chi^2/d.o.f$ = 93/80 for the \textit{Planck}xDES and ACTxDES measurements, respectively, indicating compatibility with a null signal.

%0.6532663316582915
%0.09095208777240517 1.3349149763773749 84.02219267026624 68
%/global/homes/m/mgatti/.conda/envs/py3s/lib/python3.6/site-p%ackages/ipykernel_launcher.py:95: DeprecationWarning: %elementwise comparison failed; this will raise an error in %the future.
%0.592964824120603
%0.13634824922913652 1.0968739483412056 93.95422424363593 80
